# Supplementary material for: HS-Pose: Hybrid Scope Feature Extraction for Category-level Object Pose Estimation
Source: arXiv:2303.15743 source file (2023-03-28)
Supplement: Supplementary file 1 [file corrections.tex]

\section{Important Corrections for the Paper.}
We correct some important information of the paper in here. The differences are marked in bold.
\begin{itemize}
    \item line 739 in the paper: Our method is trained us-
ing REAL275 with only 4.3k \textbf{real} images \textbf{of 18} objects while
achieving real-time performance.  
    \item line 662 (Figure 6) in the paper: The comparison of noise resistance between GPV-Pose and the proposed HS-Pose under different noise levels \textbf{(0.0\% to 40.0\% outliers)}.
    \item {\color{red}check if the deformable kernal-based graph convolution has been explained.}
\end{itemize}
